# Supplementary material for: Event-based Graph Representation with Spatial and Motion Vectors for Asynchronous Object Detection
Source: arXiv:2507.15150 source file (2025-07-20)

Raw events image

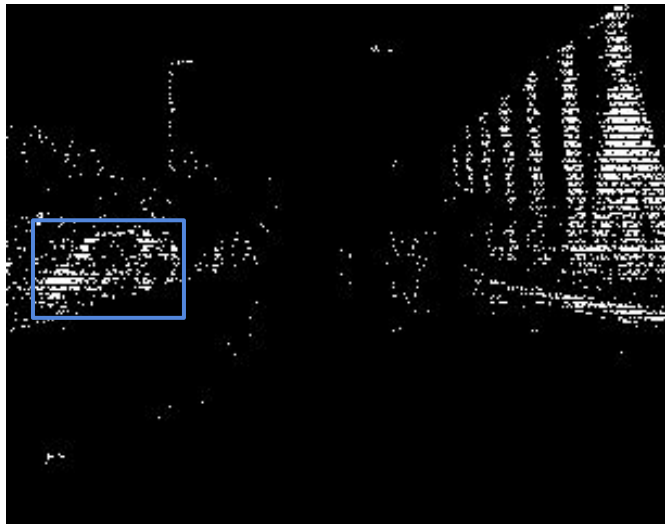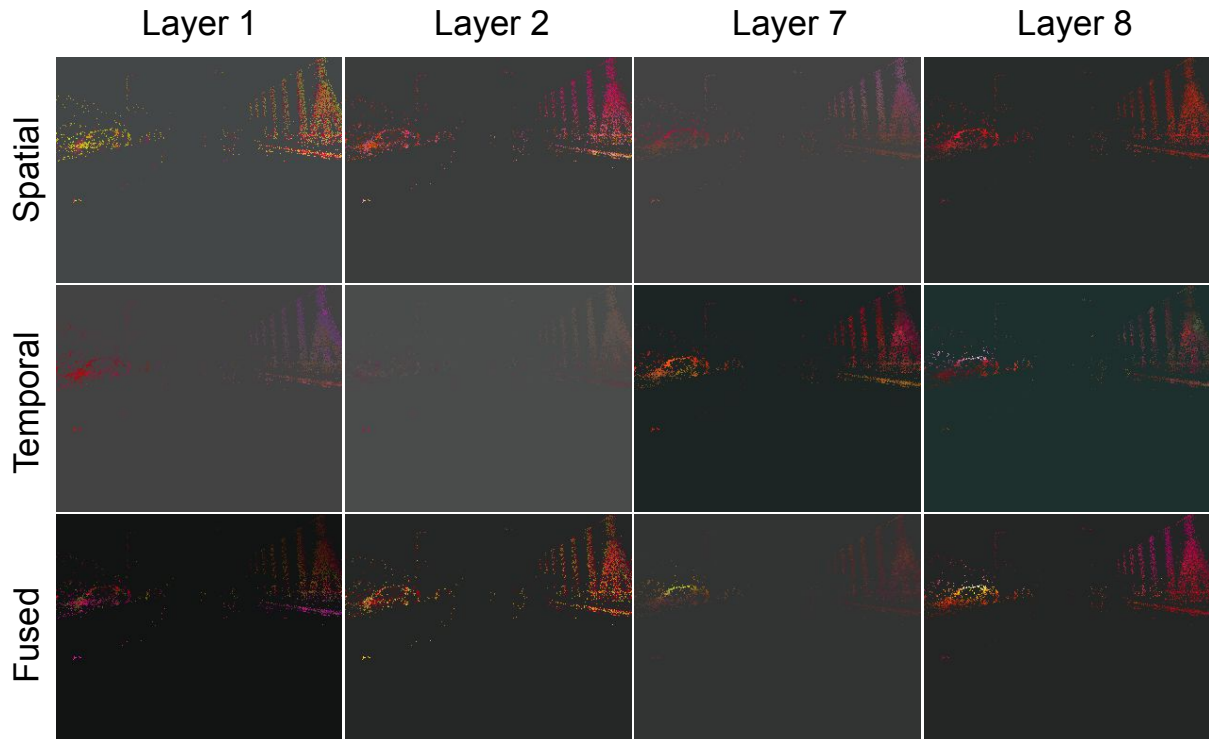

Raw events image

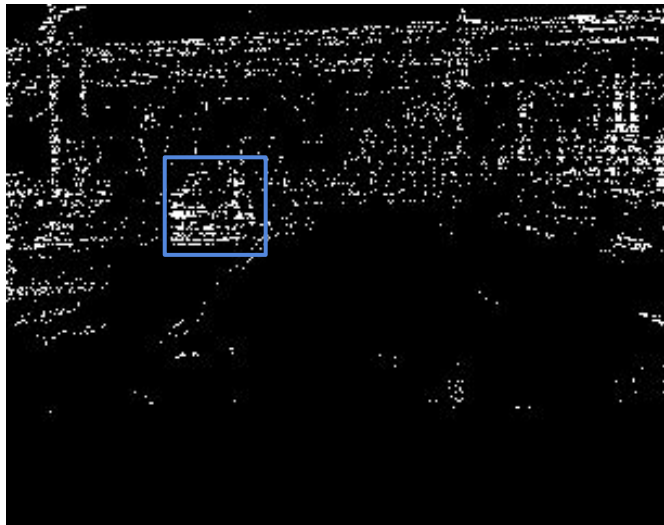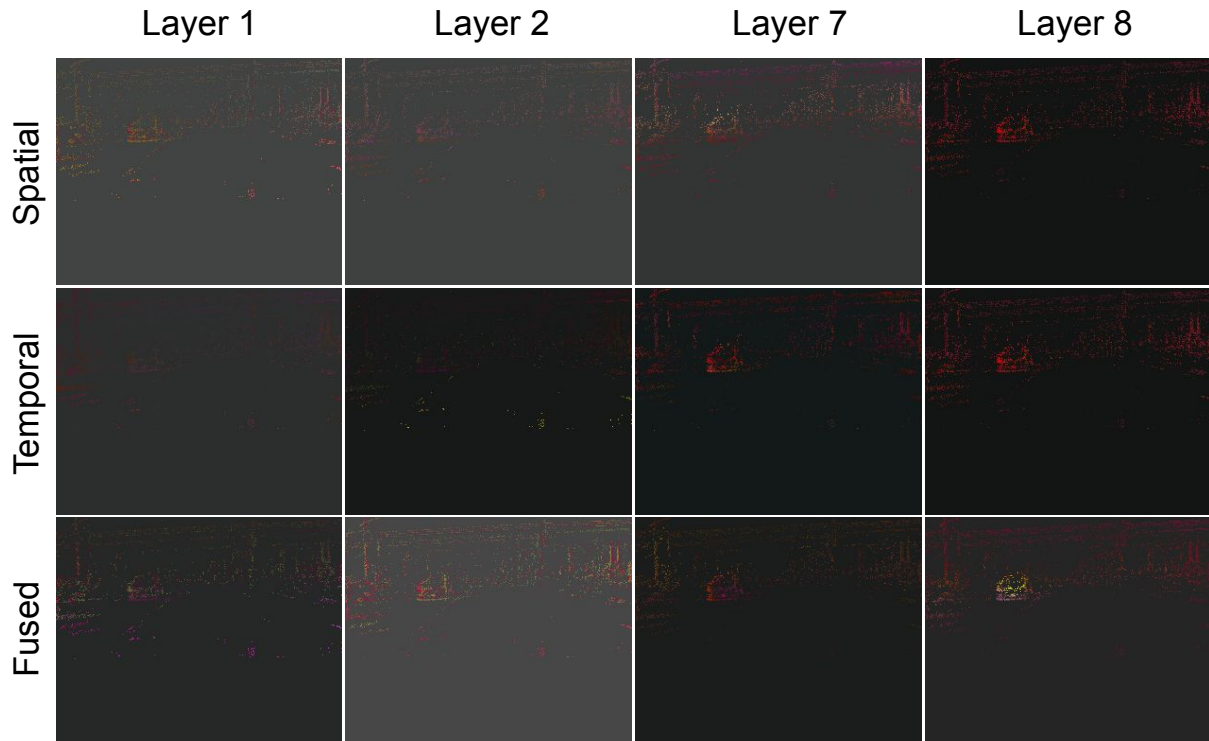

Supplement: Supplementary file 1 [file supplementary_fig3_2.pdf]
